# Supplementary material for: Entanglement induced interactions in binary mixtures
Source: arXiv:1711.05171 ancillary file (2018-07-31)
Supplement: Supplementary file 1 [file Supplemental_Material2.pdf]

# Supplemental Material for "Entanglement induced interactions in binary mixtures"

J. Chen,[1] J. M. Schurer,[1,2] and P. Schmelcher[1,2]

[1] *Zentrum für Optische Quantentechnologien, Universität Hamburg, Luruper Chaussee 149, 22761 Hamburg, Germany*

[2] *The Hamburg Centre for Ultrafast Imaging, Universität Hamburg, Luruper Chaussee 149, 22761 Hamburg, Germany*

(Dated: July 16, 2018)

This Supplemental Material for the article "Entanglement induced interactions in binary mixtures" includes the discussion of the species mean-field (SMF) approximation as well as the *ab initio* ML-MCTDHX approach. We present a detailed study on the convergence and comparison of the numerical results as well as the decomposition of the induced interactions. Moreover, we present detailed discussions on the effective state and the effects on the reduced single-species properties introduced by a small perturbation.

## I. THE SPECIES MEAN-FIELD (SMF) APPROXIMATION

The species mean-field (SMF) approximation assumes the wavefunction of the mixture to be a simple product form, i.e. $|\Psi\rangle = |\psi^A_{\rm SMF}\rangle|\psi^B_{\rm SMF}\rangle$. In order to obtain a variational optimized solution, the associated Lagrangian of the mixture is defined as

$$\mathcal{L} = \langle\Psi|\hat{H}|\Psi\rangle + \sum_{\sigma=A,B} \mu^\sigma_{\rm SMF}\left[1 - \langle\psi^\sigma_{\rm SMF}|\psi^\sigma_{\rm SMF}\rangle\right]. \quad (1)$$

where $\mu^\sigma_{\rm SMF}$ are the associated Lagrangian multiplier with the constraint of norm conservation. By varying each species function $|\psi^\sigma_{\rm SMF}\rangle$, we immediately obtain the Schrödinger-type equations for both species,

$$\left[\hat{H}_\sigma + \hat{V}^\sigma_{\rm SMF}\right]|\psi^\sigma_{\rm SMF}\rangle = \widetilde{\mu}^\sigma_{\rm SMF}|\psi^\sigma_{\rm SMF}\rangle, \quad (2)$$

with the effective Hamiltonian $\hat{H}_\sigma + \hat{V}^\sigma_{\rm SMF}$ with $\widetilde{\mu}^\sigma_{\rm SMF} = \mu^\sigma_{\rm SMF} - \langle\psi^{\bar\sigma}_{\rm SMF}|\hat{H}_{\bar\sigma}|\psi^{\bar\sigma}_{\rm SMF}\rangle$ and $\bar\sigma = B(A)$ for $\sigma = A(B)$.

The SMF induced potential is

$$\hat{V}^\sigma_{\rm SMF} = \langle\psi^{\bar\sigma}_{\rm SMF}|\hat{H}_{AB}|\psi^{\bar\sigma}_{\rm SMF}\rangle = \int dx_\sigma\ V^\sigma_{\rm SMF}(x_\sigma)\ \hat\psi^\dagger(x_\sigma)\hat\psi(x_\sigma), \quad (3)$$

with

$$V^\sigma_{\rm SMF}(x_\sigma) = \int dx_{\bar\sigma}\ H_{AB}\left(x_\sigma, x_{\bar\sigma}\right)\ \rho^{\bar\sigma}_{1-{\rm SMF}}(x_{\bar\sigma}) \quad (4)$$

and $\rho^{\bar\sigma}_{1-{\rm SMF}}(x_{\bar\sigma}) = \langle\psi^{\bar\sigma}_{\rm SMF}|\hat\psi^\dagger_{\bar\sigma}(x_{\bar\sigma})\hat\psi_{\bar\sigma}(x_{\bar\sigma})|\psi^{\bar\sigma}_{\rm SMF}\rangle$ being the SMF reduced one-body density for species $\bar\sigma$. From the Eqs. (3) and (4), we conclude that in SMF approximation the mutual impact of the species is merely an induced potential, whose profile is given by the partial trace with respect to the species $\bar\sigma$ over the interspecies interaction $H_{AB}$. In particular, for the Bose-Fermi mixture discussed in the paper, the SMF induced potential becomes $V^\sigma_{\rm SMF}(x_\sigma) = g_{bf}\rho^{\bar\sigma}_{1-{\rm SMF}}(x_\sigma)$.

## II. COMPUTATIONAL METHOD

In the *ab initio* Multi-Layer Multi-Configuration Time-Dependent Hartree method for Mixtures (ML-MCTDHX) [1–3], the state of the binary mixture $|\Psi(t)\rangle$ is first expanded as $|\Psi(t)\rangle = \sum_{i,j=1}^M A_{ij}(t)|\psi^A_i(t)\rangle|\psi^B_j(t)\rangle$, where $\{|\psi^\sigma_i(t)\rangle\}$ are the species states for $\sigma = A(B)$. Furthermore, each $|\psi^\sigma_i(t)\rangle$ is expressed in terms of number-states $|\psi^\sigma_i(t)\rangle = \sum_{\mathbf{n}|N_\sigma} C^\sigma_{i,\mathbf{n}}(t)|\mathbf{n}\rangle^\sigma_t$, where $|\mathbf{n}\rangle^\sigma_t = |n_{\sigma1}, n_{\sigma2}, \cdots\rangle$. These number-states are built by *time-dependent* single-particle functions (SPFs) $\{\phi^\sigma_k(t)\}_{k=1}^{m_\sigma}$ with particle number conservation $\sum_i n_{\sigma i} = N_\sigma$. Using the Lagrangian variational principle results in the equations of motion for the state $|\Psi(t)\rangle$ with initial value $|\Psi(0)\rangle$. It should be pointed out that both coefficients $A_{ij}(t)$ and $C^\sigma_{i,\mathbf{n}}(t)$ as well as the SPFs $\phi^\sigma_k(t)$ are variationally optimized in the dynamical evolution. Moreover, by means of an improved relaxation method based on imaginary time propagation [4], the ML-MCTDHX makes it possible to also determine stationary states (ground and excited states).

The $m_\sigma$ and $M$ are the main numerical control parameters, in which $m_\sigma$ truncates the dimension of the single-particle Hilbert space, leading to a species space of size $K_\sigma = \begin{pmatrix} N_\sigma + m_\sigma - 1 \\ m_\sigma - 1 \end{pmatrix}$ $\left[K_\sigma = \begin{pmatrix} m_\sigma \\ N_\sigma \end{pmatrix}\right]$ for $N_\sigma$ bosons (fermions), while $M \leqslant \min\{K_A, K_B\}$ defines that only $M$ species states are used to construct the full many-body Hilbert space.

Finally, we obtain the Schmidt numbers and Schmidt states by diagonalizing the reduced density matrix for species $\sigma$. We emphasize that for $M = 1$ the simulations of ML-MCTDHX coincide with the species mean-field (SMF) approximation. For $M = \min\{K_A, K_B\}$, the so-called full configuration interaction (CI), all possible number-state configurations are considered.

## III. CONVERGENCE AND DECOMPOSITION OF THE INDUCED INTERACTIONS

For the Bose-Fermi mixture discussed in the paper, the induced interaction is given by

$$H^\sigma_{\rm ind}(x_1, x_2) = g_{bf} \sum_{i\neq 1} \frac{2\sqrt{\lambda_i}}{\tilde{t}_{1i}} \gamma^{\bar{\sigma}}_{1i}(x_1)\gamma^{\bar{\sigma}}_{i1}(x_2), \tag{5}$$

where $g_{bf}$ is the Bose-Fermi interaction strength, $\lambda_i$ the Schmidt numbers, $\gamma^{\bar{\sigma}}_{1i}(x) = \langle\psi^{\bar{\sigma}}_1|\hat{\psi}^\dagger_{\bar{\sigma}}(x)\hat{\psi}_{\bar{\sigma}}(x)|\psi^{\bar{\sigma}}_i\rangle$, and $\tilde{t}_{1i} = \int dx\ \gamma^\sigma_{1i}(x)\gamma^{\bar{\sigma}}_{1i}(x)$. In order to obtain a converged induced interaction, we inspect the convergence of all the Schmidt numbers $\lambda_i$ as well as of the $\gamma^\sigma_{1i}(x)$. First, we compare the simulations with fixed number of SPFs, i.e. $m_f = m_b = m$, and vary the species state number $M$. Once we have obtained convergence with respect to $\lambda_i$ and $\gamma^\sigma_{1i}(x)$, we increase the number of SPFs and check the convergence by means of the same procedure. Finally, we compare the results for different $m$. In the following discussion, we label the parameter configuration as M-(m) which refers to the simulation with $M$ species states and $m$ SPFs. Moreover, we use the interaction strength $g_{bf} = 1.0$ as discussed in the paper.

*a. Convergence of the Schmidt numbers* Let us begin with the convergence of the Schmidt numbers. As aforementioned, we first compare the results for fixed m and vary the number of species states $M$. An exemplary result is presented in the Supp-Fig. 1(a), with $m = 10$ and $M = 10, 11, 12$. For increasing the number of species states, the corresponding values are almost indistinguishable (see blue, red and black lines, respectively). To quantitatively demonstrate the convergence, we introduce the relative difference of the $i$-th Schmidt number as $\delta\lambda^{CC'}_i = |\lambda^C_i - \lambda^{C'}_i|/\lambda^{C'}_i$ [1], where $\lambda^C_i$ ($\lambda^{C'}_i$) denotes the $i$-th Schmidt number calculated with the C = M-(m) [C$'$ = M$'$-(m$'$)] configuration. We notice that for increasing $M$ the relative difference decreases significantly [c.f. Supp-Fig. 1(c)]. In particular, for the comparison of the C = 11-(10) and C$'$ = 12-(10) simulations, the maximum deviation of the first ten Schmidt numbers is less than 0.5%.

Next, we compare the simulations for different m. The computed Schmidt numbers as well as the relative differences are shown in Supp-Fig. 1(b) and (d), respectively, where $M = 12$ and $m = 8, 9, 10$. From the comparison between the C = 12-(9) and C$'$ = 12-(10) simulations, we find that the values of the first eight Schmidt numbers show a good agreement, with a maximal relative deviation of less than 6%. For the higher-order Schmidt numbers ($i \geqslant 9$), although the relative deviations exceed 20%, their absolute values are less than $10^{-4}$ [c.f. Supp-Fig. 1(b)].

*b. Convergence of the* $\gamma^\sigma_{1i}$ The computed $\gamma^\sigma_{1i}$ for $m = 10$ and $M = 10, 11, 12$ are presented in Supp-Fig. 2, where, as an exemplary result, the profiles of $\gamma^\sigma_{12}, \gamma^\sigma_{16}, \gamma^\sigma_{1-10}$ are depicted for fermionic (upper panels) and bosonic (lower panels) species, respectively. From those figures we can not find any significant differences. In order to quantitatively judge the convergence, we inspect the relative spatially integrated difference $[\Delta^{CC'}_i]_\sigma = \frac{1}{N_\sigma}\left[\frac{\int dx\ |\gamma^C_i(x) - \gamma^{C'}_i(x)|}{\int dx\ |\gamma^{C'}_i(x)|}\right]_\sigma$, where $N_\sigma$ is the particle number for species $\sigma$. For increasing $M$, we find the relative spatially integrated differences to significantly decrease (results not shown here), in particular, for the comparison of the 11-(10) and 12-(10) simulations, the maximum deviation is less than 0.1% for the first nine $\gamma^\sigma_{1i}$ (from $\gamma^\sigma_{12}$ to $\gamma^\sigma_{1-10}$) and reaches about 2% for $\gamma^\sigma_{1-11}$.

Next, we compare the results for different $m$. In Supp-Fig. 3 and 4, we present the $\gamma^\sigma_{1i}$ for both species as a result of 12-(8) (red dashed lines), 12-(9) (blue solid lines) and 12-(10) (green dash-dot lines) simulations, respectively. We notice that the results for these three configurations show a good agreement from $\gamma^\sigma_{12}$ to $\gamma^\sigma_{18}$, while large deviations occur for $\gamma^\sigma_{19}$ for the comparison of the 12-(8) and 12-(9) simulations. Once we increase the number of SPFs, the difference dramatically reduces [c.f. Supp-Fig. 3, 4, (h) blue solid line and green dashed-dot line]. However, for the last three $\gamma^\sigma_{1i}$, all of those results show large deviations. This is quantitatively characterised by the aforementioned relative spatially integrated differences $[\Delta^{CC'}_i]_\sigma$, for which we observe a maximum deviation of the order of 5% for the first seven $\gamma^\sigma_{1i}$ (from $\gamma^\sigma_{12}$ to $\gamma^\sigma_{18}$), while it ranges from 15% to 50% for the last four $\gamma^\sigma_{1i}$.

Once we have obtained the $\gamma^\sigma_{1i}$, the associate denominators $\tilde{t}_{1i}$ in Eq. (5) can be readily calculated. In Supp-Fig. 5(a), we present those values of the simulations with $m = 10$ and $M = 10, 11, 12$. With increasing number of

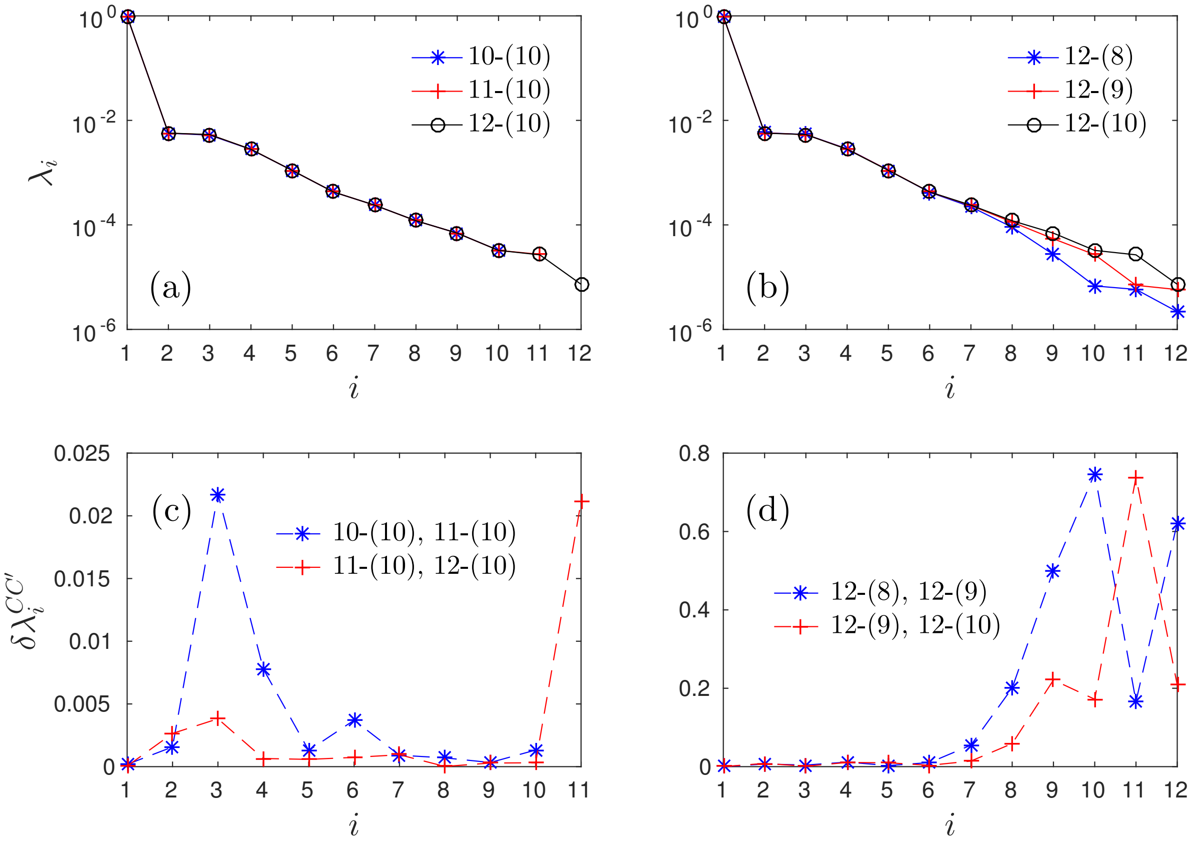


Supp-Fig. 1. The upper panels represent Schmidt numbers for different parameter configurations with ML-MCTDHX simulations: (a) $m = 10$ and $M = 10, 11, 12$, (b) $M = 12$ and $m = 8, 9, 10$. The lower panels are the corresponding relative differences.

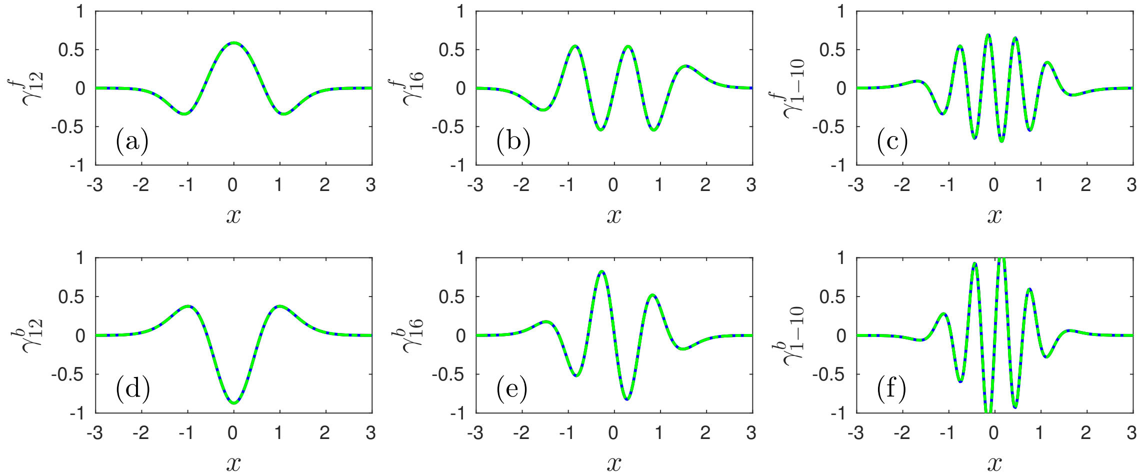


Supp-Fig. 2. $\gamma_{1i}^{\sigma}$ for $m = 10$ and $M = 10$ (red dashed line), $M = 11$ (blue solid line) as well as $M = 12$ (green dashed-dot line) ML-MCTDHX simulations for fermionic (upper panels) and bosonic (lower panels) species, respectively.

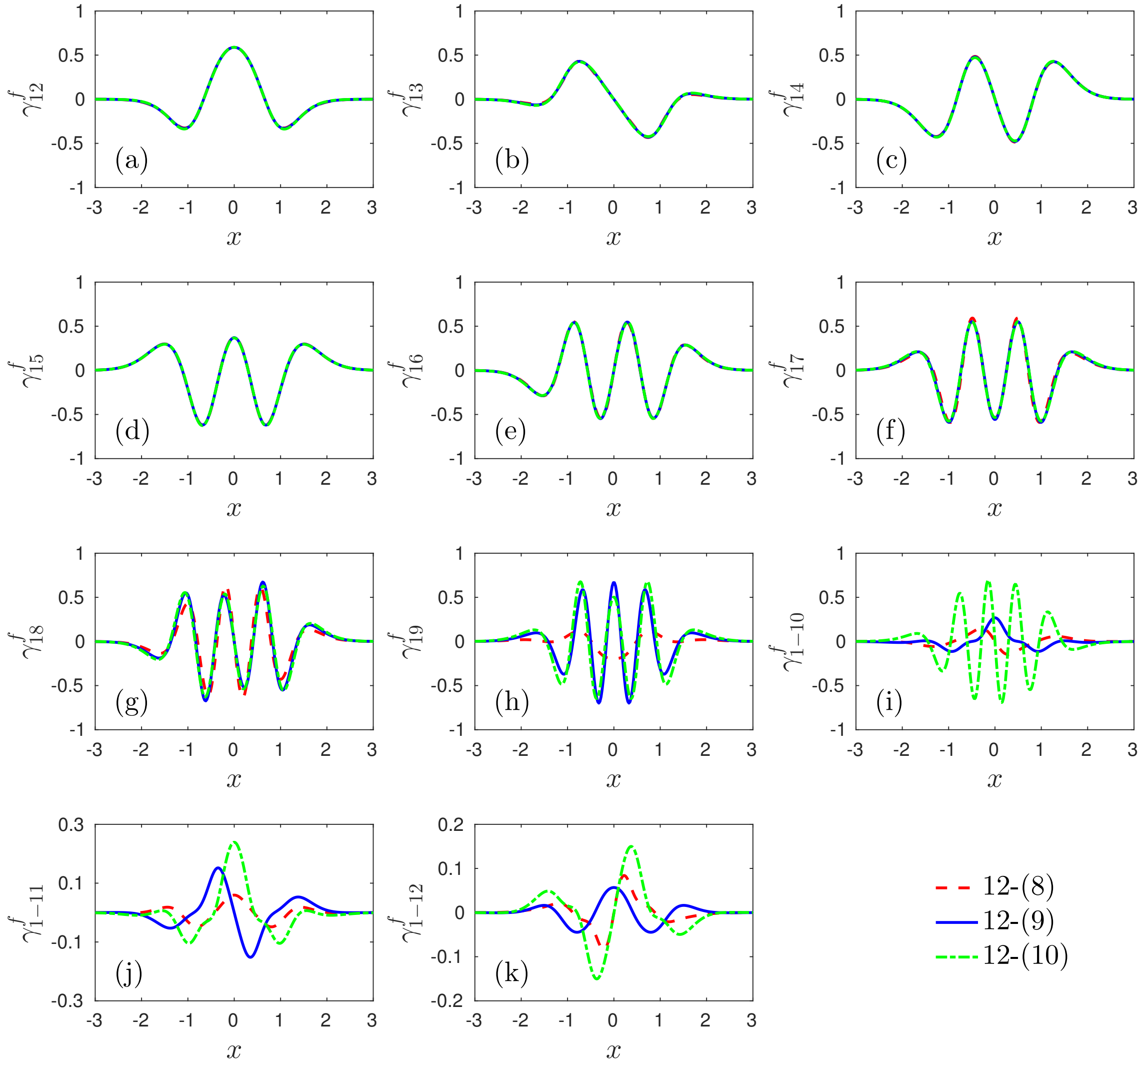


Supp-Fig. 3. $\gamma^f_{1i}$ for 12-(8) (red dashed lines), 12-(9) (blue solid lines) as well as 12-(10) (green dashed-dot lines) ML-MCTDHX simulations.

species states, we find that the values of $\tilde{t}_{1i}$ become more or less the identical. The comparison for different $m$ is depicted in Supp-Fig. 5(b). For different $m$, those higher-order $\tilde{t}_{1i}$ are changed dramatically. For instance, $\tilde{t}_{19} \approx 0$ for $m = 8$, however, changes abruptly to $\tilde{t}_{19} \approx -0.55$ for $m = 9, 10$. As we discussed before, this behaviour directly stems from the large deviations of the associated $\gamma^{\sigma}_{1i}$. However, we also witness that the first seven $\tilde{t}_{1i}$, to a good accuracy, remain the same.

*c. Construction of the induced interactions* To construct the induced interactions, we first have to exclude the terms for $\tilde{t}_{1i} = 0$ [see Eq. (5)], since the corresponding interaction $[2\sqrt{\lambda_i}\gamma^{\bar{\sigma}}_{1i}(x_1)\gamma^{\bar{\sigma}}_{i1}(x_2)/\tilde{t}_{1i}]$ is divergent. Moreover, by comparing the results for different numbers of SPFs, we notice that for both the Schmidt numbers and the $\gamma^{\sigma}_{1i}$, those high-order terms ($i \geqslant 9$) have large deviations. Therefore, in order to construct the convergent induced interactions, we have to truncate the sum over $i$ to $P_{cut}$ in Eq. (5). In the maintext, we chose $P_{cut} = 8$.

*d. Comparison to Exact Diagonalization (ED)* The computed $\gamma^{\sigma}_{1i}$ using exact diagonalization (ED) are presented in Supp-Fig. 6 (red solid lines) for $m = 12$ (full CI) for both fermionic (upper panels) and bosonic (lower panels) species. Note that here we take the eigenstates of the harmonic oscillator as the SPFs for the ED simulations. For comparison,

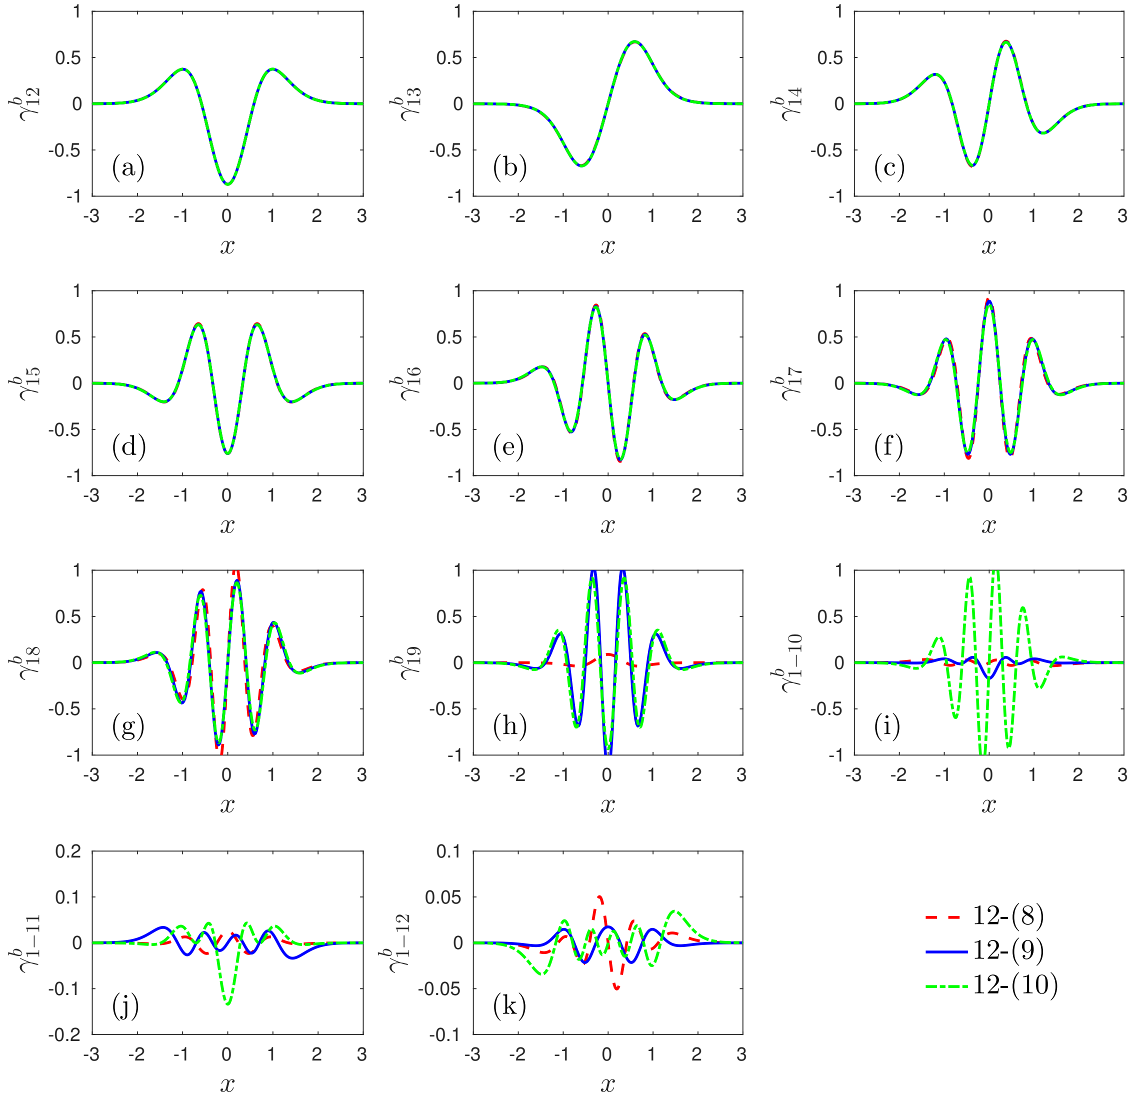


Supp-Fig. 4. $\gamma^b_{1i}$ for 12-(8) (red dashed lines), 12-(9) (blue solid lines) as well as 12-(10) (green dashed-dot lines) ML-MCTDHX simulations.

we depict the profiles from the ML-MCTDHX simulations with 12-(10) as well. We observe that, the results of both methods possess a quantitative agreement from $\gamma^\sigma_{12}$ to $\gamma^\sigma_{14}$, with a maximum relative difference $[\Delta^{CC'}_i]_\sigma \approx 6\%$ (results not shown here), however, for $i \geqslant 5$ the deviations become large, for instance, $[\Delta^{CC'}_6]_\sigma \approx 30\%$ The above comparison indicates the exact diagonalization can quantitatively capture the profiles of the induced interactions, however, it becomes inefficient to depict the high-order $\gamma^\sigma_{1i}$ [we observe that for increasing the number of SPFs, the profiles of high-order $\gamma^\sigma_{1i}$ are much closer to the ML-MCTDHX simulations (results not shown here)].

*e. Decompositions of the induced interactions* Eq. (5) not only introduces the methodology for constructing the induced interaction but also provides the possibility for investigating the induced interaction with respect to the contribution of each Schmidt state. The decomposition of the induced interaction among the fermions (bosons) is shown in Supp-Fig. 7 (Supp-Fig. 8), in which (a) is the induced interaction itself, (b-h) are the contributions made by the corresponding Schmidt states, i.e. the term $[2g_{bf}\sqrt{\lambda_i}\gamma^{\bar{\sigma}}_{1i}(x_1)\gamma^{\bar{\sigma}}_{i1}(x_2)]/\tilde{t}_{1i}$ $(i \geqslant 2)$. From this decomposition,

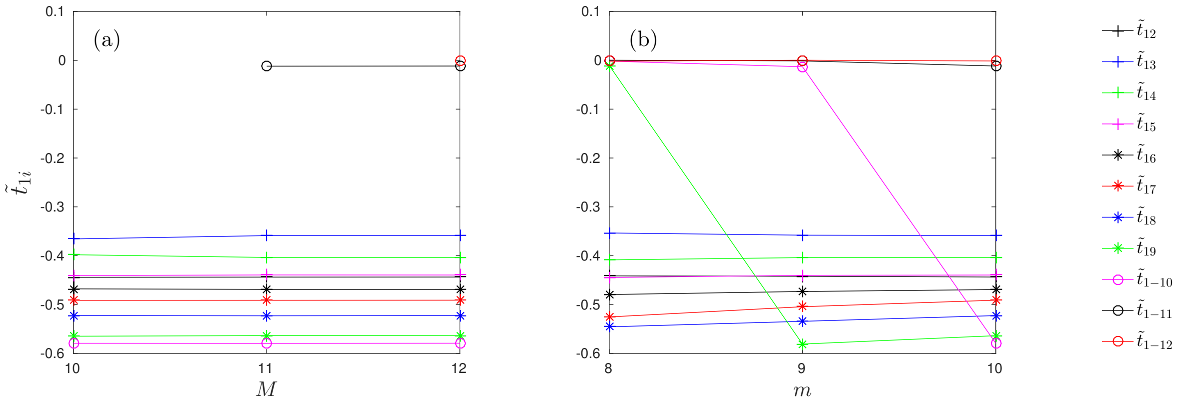


Supp-Fig. 5. (a) $\tilde{t}_{1i}$ for fixed $m = 10$ and varying number of species states $M = 10, 11, 12$. (b) $\tilde{t}_{1i}$ for 12-(8), 12-(9) and 12-(10) simulations.

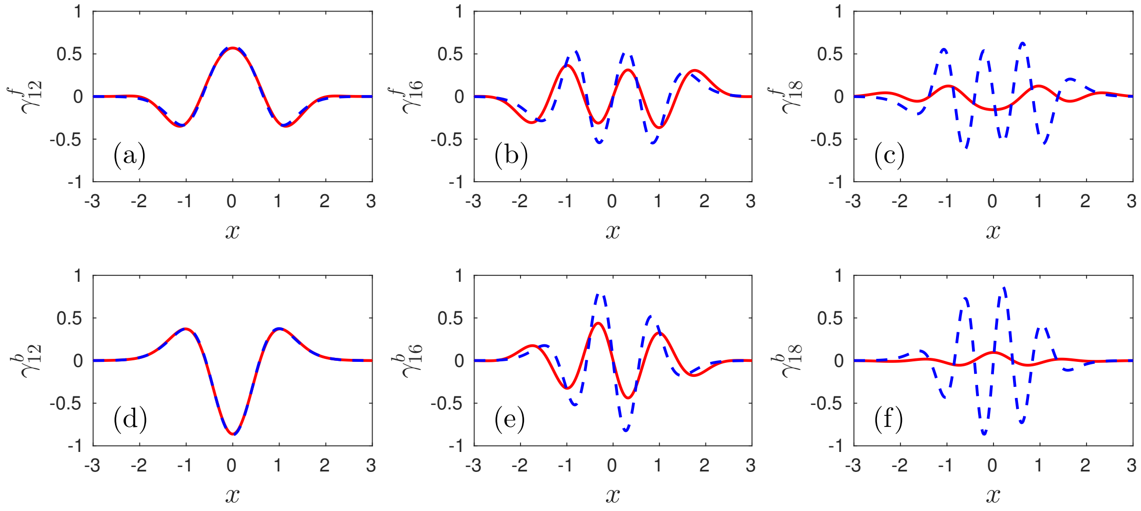


Supp-Fig. 6. Comparison of $\gamma^\sigma_{1i}$: exact diagonalization (red solid lines) and ML-MCTHDX (blue dashed lines) for fermionic (upper panels) and bosonic (lower panels) species, respectively.

we observe that, due to the pre-factors $\sqrt{\lambda_i}$, the intensity of each term monotonously decreases with increasing $i$, indicating that the contributions for those higher-order Schmidt states are negligible. Interestingly, we also find, although the pattern of each component highly depends on both the relative coordinate $r = x_1 - x_2$ as well as the center-of-mass coordinate $R = (x_1 + x_2)/2$, the final form of the induced interaction mainly depends on the relative distance between the two particles.

## IV. DISCUSSIONS OF EFFECTIVE STATE AND PERTURBATIONS

For a give eigenstate $|\Psi\rangle$ of the mixture, we derive an effective single-species Hamiltonian

$$\hat{H}^\sigma_{\text{eff}} = H^{\bar{\sigma}}_{11} + \sum_{i\neq 1} \frac{\sqrt{\lambda_i} H^{\bar{\sigma}}_{1i} H^{\bar{\sigma}}_{i1}}{t_{1i}}, \tag{6}$$

and the associated effective Schrödinger equation $\hat{H}^\sigma_{\text{eff}}|\psi^\sigma_{\text{eff}}\rangle = E^\sigma_{\text{eff}}|\psi^\sigma_{\text{eff}}\rangle$, with $|\psi^\sigma_{\text{eff}}\rangle$ being an eigenstate of $\hat{H}^\sigma_{\text{eff}}$. On the other hand, an overall perturbation acting on the mixture will change the structure of the wavefunction $|\Psi\rangle$ to some extend which, in turn, impacts the effective single-species physics leading to modifications of, e.g., the reduced

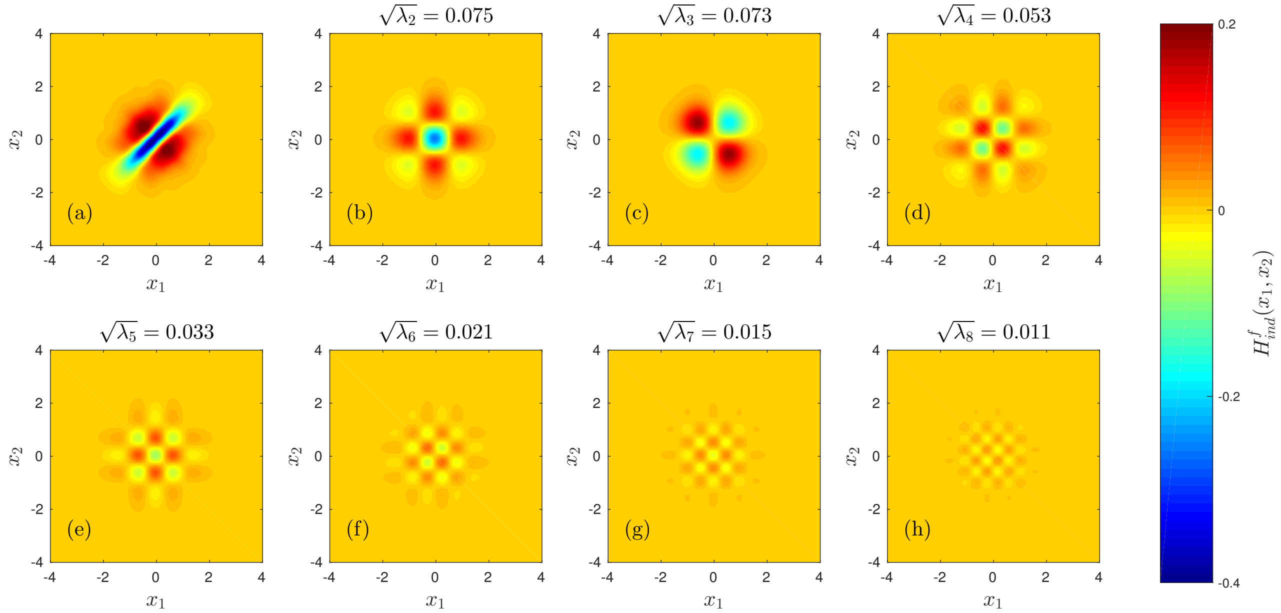


Supp-Fig. 7. (a) Fermionic induced interaction, (b-h) the contributions of the corresponding Schmidt states.

density matrix and the effective Hamiltonian. In the following, we discuss the effective state $|\psi^\sigma_{\text{eff}}\rangle$ in more detail and investigate how a small perturbation affects the reduced single-species properties.

*a. Effective state* As mentioned in the main text, the effective state $|\psi^\sigma_{\text{eff}}\rangle$ is an eigenstate of $\hat{H}^\sigma_{\text{eff}}$ whose eigenvalue $E^\sigma_{\text{eff}}$ is closest to $E^\sigma_1 = \langle\psi^\sigma_1|\hat{H}^\sigma_{\text{eff}}|\psi^\sigma_1\rangle$. To gain further insights, let us first project onto the $q$-th Schmidt state $\langle\psi^{\bar{\sigma}}_q|$, which gives rise to

$$\lambda_1 H^{\bar{\sigma}}_{11}|\psi^\sigma_1\rangle + \sum_{i\neq 1}\sqrt{\lambda_1}\sqrt{\lambda_i}H^{\bar{\sigma}}_{1i}|\psi^\sigma_i\rangle = \mu_1|\psi^\sigma_1\rangle, \tag{7}$$

$$|\psi^\sigma_q\rangle = M_q\sum_{j\neq q}\sqrt{\lambda_j}\sqrt{\lambda_q}H^{\bar{\sigma}}_{qj}|\psi^\sigma_j\rangle \qquad (q>1), \tag{8}$$

with $H^{\bar{\sigma}}_{ij} = \langle\psi^{\bar{\sigma}}_i|\hat{H}|\psi^{\bar{\sigma}}_j\rangle$ and $M_q = \left[\mu_q - \lambda_q H^{\bar{\sigma}}_{qq}\right]^{-1}$. Substituting Eq. (8) into both sides of Eq. (7) yields the expression

$$\lambda_1 H^{\bar{\sigma}}_{11}|\psi^\sigma_1\rangle + \sum_{i\neq 1}\sum_{j\neq i}\sqrt{\lambda_1}\lambda_i\sqrt{\lambda_j}H^{\bar{\sigma}}_{1i}M_i H^{\bar{\sigma}}_{ij}|\psi^\sigma_j\rangle = \mu_1|\psi^\sigma_1\rangle, \tag{9}$$

with $\mu_1 = \sum_i\sum_{j\neq i}\sqrt{\lambda_1}\lambda_i\sqrt{\lambda_j}\langle\psi^\sigma_1|H^{\bar{\sigma}}_{1i}M_i H^{\bar{\sigma}}_{ij}|\psi^\sigma_j\rangle$.

In the weak-entanglement regime, all $\sqrt{\lambda_{i\neq 1}}$ are assumed to be of order $\delta$ with $\delta \ll 1$. Equipped with this knowledge, Eq. (9) can be rewritten as a power series of $\delta$

$$\hat{H}^\sigma_{\text{eff}}|\psi^\sigma_1\rangle + K^\sigma = (E^\sigma_1 + E^\sigma_2)|\psi^\sigma_1\rangle, \tag{10}$$

where $\hat{H}^\sigma_{\text{eff}}|\psi^\sigma_1\rangle$ and $E^\sigma_1|\psi^\sigma_1\rangle$ contain all the zeroth and the first order terms of $\delta$, while $K^\sigma$ and $E^\sigma_2$ are of $O(\delta^2)$. Eq. (10) indicates that for the limit $\lambda_{i\neq 1}\to 0$, $\forall i$, it is possible to find an eigenstate of $\hat{H}^\sigma_{\text{eff}}$ which resembles $|\psi^\sigma_1\rangle$ the closest, while, at the same time, its eigenvalue $E^\sigma_{\text{eff}}$ is also closest to $E^\sigma_1$. For the case that $E^\sigma_{\text{eff}}$ is degenerate, one shall select the eigenstate which has maximal overlap with $|\psi^\sigma_1\rangle$. Furthermore, we note that for the Bose-Fermi mixture, $|\psi^\sigma_{\text{eff}}\rangle$ is the ground state of $\hat{H}^\sigma_{\text{eff}}$.

*b. Small perturbations acting on the mixture* Let us denote $\hat{H}_0$ as the Hamiltonian for the unperturbed mixture, whose eigenvalues and eigenstates are known via $\hat{H}_0|\Psi^{(0)}_n\rangle = E^{(0)}_n|\Psi^{(0)}_n\rangle$. Without loss of generality, we assume that the spectrum of $\hat{H}_0$ is discrete and non-degenerate. In the following, we consider the case where the unperturbed

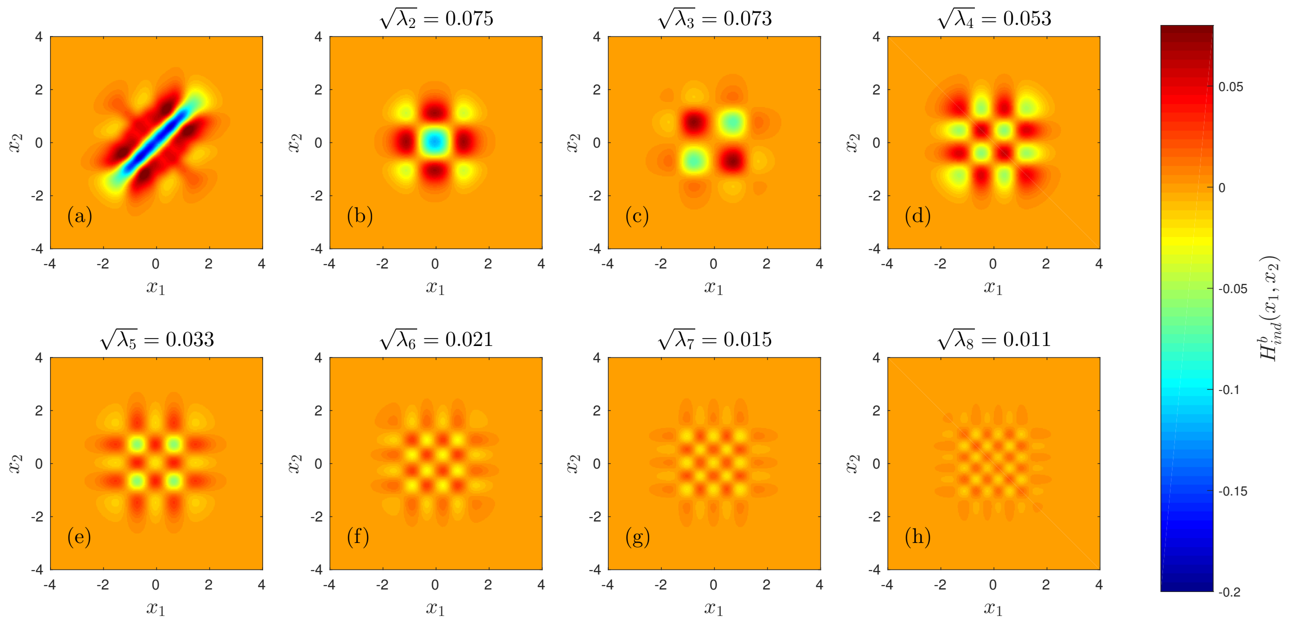


Supp-Fig. 8. (a) Bosonic induced interaction, (b-h) the contributions of the corresponding Schmidt states.

mixture is in the $m$-th eigenstate $|\Psi_m^{(0)}\rangle$ being weakly interspecies entangled and investigate how a small perturbation of $\hat{H}_0$ affects the reduced single-species properties. It is worth to note that both the unperturbed state $|\Psi_m^{(0)}\rangle$ and the perturbed state $|\Psi_m\rangle$ can be written in the form $|\Psi_m^{(0)}\rangle = \sum_i \sqrt{\lambda_i}|\psi_i^A\rangle|\psi_i^B\rangle$ and $|\Psi_m\rangle = \sum_i \sqrt{\xi_i}|\phi_i^A\rangle|\phi_i^B\rangle$ via Schmidt decompositions. Moreover, we denote $\hat{\rho}_\sigma$ ($\hat{\rho}_\sigma^{(0)}$) being the perturbed (unperturbed) reduced $\sigma$-species density matrix. The main results include then the following: (i) The perturbed reduced density matrix $\hat{\rho}_\sigma$ resembles $\hat{\rho}_\sigma^{(0)}$. (ii) The perturbed state $|\Psi_m\rangle$ is still weakly entangled whose first Schmidt state $|\phi_1^\sigma\rangle$ is close to the unperturbed one ($|\psi_i^\sigma\rangle$). (iii) The term $H_{11}^\sigma$ in the effective Hamiltonian is robust against perturbations.

For the perturbed Hamiltonian $\hat{H} = \hat{H}_0 + g\hat{V}$, the $m$-th eigenstate (up to the first-order correction) is

$$|\Psi_m\rangle = |\Psi_m^{(0)}\rangle - \sum_{k\neq m} \frac{\langle\Psi_k^{(0)}|g\hat{V}|\Psi_m^{(0)}\rangle}{E_k^{(0)} - E_m^{(0)}}|\Psi_k^{(0)}\rangle = |\Psi_m^{(0)}\rangle - \sum_{k\neq m} V_{km}|\Psi_k^{(0)}\rangle, \tag{11}$$

with $g\hat{V}$ being the perturbation and $g$ is a parameter used for the corresponding power expansion. Here $V_{km} = \frac{\langle\Psi_k^{(0)}|g\hat{V}|\Psi_m^{(0)}\rangle}{E_k^{(0)} - E_m^{(0)}}$ is of $O(g)$ and we note that the applicability of perturbation theory requires $|V_{km}| \ll 1$. On the other hand, the Schmidt states $\{|\psi_i^\sigma\rangle\}$ for $|\Psi_m^{(0)}\rangle$ form an orthonormal basis, therefore, we can expand $|\Psi_k^{(0)}\rangle$ as

$$|\Psi_k^{(0)}\rangle = \sum_{\alpha\beta} C_{\alpha\beta}^k |\psi_\alpha^A\rangle|\psi_\beta^B\rangle. \tag{12}$$

Substituting Eq. (12) into Eq. (11) yields the expression

$$|\Psi_m\rangle = |\Psi_m^{(0)}\rangle - \sum_{\alpha\beta} T_{\alpha\beta}|\psi_\alpha^A\rangle|\psi_\beta^B\rangle, \tag{13}$$

with $T_{\alpha\beta} = \sum_{k\neq m} V_{km} C_{\alpha\beta}^k$ being of $O(g)$.

Accordingly, the perturbed reduced density matrix becomes

$$\hat{\rho}_\sigma = tr_{\bar{\sigma}}|\Psi_m\rangle\langle\Psi_m| = \hat{\rho}_\sigma^{(0)} - \sum_{ij}[\sqrt{\lambda_i}T_{ji} + \sqrt{\lambda_j}T_{ij}]|\psi_i^\sigma\rangle\langle\psi_j^\sigma| + \sum_{ij\alpha} T_{i\alpha}T_{j\alpha}|\psi_i^\sigma\rangle\langle\psi_j^\sigma| \approx \hat{\rho}_\sigma^{(0)} - \hat{\rho}_\sigma^{(1)}, \tag{14}$$

with $\hat{\rho}_\sigma^{(0)} = \sum_i \lambda_i |\psi_i^\sigma\rangle\langle\psi_i^\sigma|$ ($\lambda_1 > \lambda_2 > \cdots$) being the unperturbed reduced density matrix and

$$\hat{\rho}_\sigma^{(1)} = \sum_{ij} [\sqrt{\lambda_i} T_{ji} + \sqrt{\lambda_j} T_{ij}] |\psi_i^\sigma\rangle\langle\psi_j^\sigma| = \sum_{ij} [\rho_\sigma^{(1)}]_{ij} \, |\psi_i^\sigma\rangle\langle\psi_j^\sigma| \tag{15}$$

is the first-order correction in which $|[\rho_\sigma^{(1)}]_{ij}| \ll 1$ [being of $O(g)$]. From Eq. (14), we conclude that the perturbed reduced density matrix $\hat{\rho}_\sigma$ can be expanded in a power series of $g$ where $\hat{\rho}_\sigma^{(0)}$ is the zeroth-order term. For the case $V_{km} \to 0$, we have $\hat{\rho}_\sigma \to \hat{\rho}_\sigma^{(0)}$.

Next, let us discuss the Schmidt numbers and Schmidt states for the perturbed state $|\Psi_m\rangle$. It is important to note that, for a strongly entangled unperturbed state $|\Psi_m^{(0)}\rangle$ the values of its Schmidt numbers $(\lambda_1, \lambda_2, \cdots)$ can be arbitrarily close to each other. Hence, the term $\hat{\rho}_\sigma^{(1)}$ in Eq.(14) can no longer be treated as a perturbation. In contrast, for the case where $|\Psi_m^{(0)}\rangle$ is weakly entangled, the first Schmidt number as well as the first Schmidt state for the perturbed state $|\Psi_m\rangle$ can still be obtained perturbatively, due to the presence of large difference between $\lambda_1$ and all $\lambda_{i\neq 1}$. Equipped with this knowledge, we have

$$\xi_1 = \lambda_1 + [\rho_\sigma^{(1)}]_{11}, \tag{16}$$

$$\begin{aligned} |\phi_1^\sigma\rangle &= |\psi_1^\sigma\rangle - \sum_{k\neq 1} \frac{[\rho_\sigma^{(1)}]_{k1}}{\lambda_k - \lambda_1} |\psi_k^{(0)}\rangle \\ &\approx |\psi_1^\sigma\rangle - \sum_{k\neq 1} \frac{[\rho_\sigma^{(1)}]_{k1}}{\lambda_1} |\psi_k^\sigma\rangle = |\psi_1^\sigma\rangle - \sum_{k\neq 1} \varrho_k^\sigma |\psi_k^\sigma\rangle. \end{aligned} \tag{17}$$

Importantly, the restriction $|\varrho_k^\sigma| = |\frac{[\rho_\sigma^{(1)}]_{k1}}{\lambda_1}| \ll 1$ can be naturally fulfilled, since $|[\rho_\sigma^{(1)}]_{k1}| \ll 1$ and $\lambda_1 \approx 1$. In this sense, we conclude that the perturbed state $|\Psi_m\rangle$ still remains weakly entangled whose first Schmidt number $\xi_1 \approx \lambda_1$ and the first Schmidt state $|\phi_1^\sigma\rangle$ is close to $|\psi_1^\sigma\rangle$. Moreover, we obtain

$$|\phi_1^\sigma\rangle\langle\phi_1^\sigma| \approx |\psi_1^\sigma\rangle\langle\psi_1^\sigma| - \sum_{k\neq 1} \frac{[\rho_\sigma^{(1)}]_{k1}}{\lambda_1} |\psi_k^\sigma\rangle\langle\psi_1^\sigma| - \sum_{k\neq 1} \frac{[\rho_\sigma^{(1)}]_{k1}}{\lambda_1} |\psi_1^\sigma\rangle\langle\psi_k^\sigma|. \tag{18}$$

Compared with Eq. (18) and Eq. (14) and by noticing $[\rho_\sigma^{(1)}]_{1k} = [\rho_\sigma^{(1)}]_{k1} \gg [\rho_\sigma^{(1)}]_{\alpha\beta}$ for $\alpha, \beta \neq 1$, we conclude that the perturbed density matrix $\hat{\rho}_\sigma$ is dominated by the first Schmidt state $|\phi_1^\sigma\rangle$, which is similar to the unperturbed case.

The last important observation is that the first term $H_{11}^{\bar{\sigma}}$ in the effective Hamiltonian is robust against perturbations [see Eq. (6)]. For the perturbed state, $H_{11}^{\bar{\sigma}}$ becomes

$$H_{11}^{\bar{\sigma}} = \langle\phi_1^{\bar{\sigma}}|\hat{H}|\phi_1^{\bar{\sigma}}\rangle \approx \langle\psi_1^{\bar{\sigma}}|\hat{H}_0|\psi_1^{\bar{\sigma}}\rangle + \langle\psi_1^{\bar{\sigma}}|g\hat{V}|\psi_1^{\bar{\sigma}}\rangle - \sum_{i\neq 1} [\varrho_i^\sigma \langle\psi_1^{\bar{\sigma}}|\hat{H}_0|\psi_i^{\bar{\sigma}}\rangle + c.c.] \tag{19}$$

with $c.c$ being the complex conjugate. Here, we note that $\langle\psi_1^{\bar{\sigma}}|\hat{H}_0|\psi_1^{\bar{\sigma}}\rangle$ is the unperturbed part, $\langle\psi_1^{\bar{\sigma}}|g\hat{V}|\psi_1^{\bar{\sigma}}\rangle$ and $\sum_{i\neq 1}[\varrho_i^\sigma \langle\psi_1^{\bar{\sigma}}|\hat{H}_0|\psi_i^{\bar{\sigma}}\rangle + c.c.]$ are of $O(g)$ while the terms of $O(g^2)$ are neglected. From Eq. (19), we clearly see that $H_{11}^{\bar{\sigma}}$ is close to $\langle\psi_1^{\bar{\sigma}}|\hat{H}_0|\psi_1^{\bar{\sigma}}\rangle$ for a small perturbation which manifests its robustness. Moreover, $H_{11}^{\bar{\sigma}}$ is also the dominant term among the effective Hamiltonian, since we have $\sqrt{\lambda_i} \ll 1$ for $i \neq 1$ for the weak-entanglement regime.

*c. Robustness of induced interaction* Let us discuss the variations of both the induced potential and the induced interaction introduced by the perturbations. To this end, we investigate the changes of the $\gamma_{1i}^\sigma$ for both species, since they completely determine the spatial profiles of the induced interaction and induced potential [c.f. Eqs. (14-16) in the main text]. We now introduce three types of perturbations, which are the changes of Bose-Bose ($g_b$), Bose-Fermi ($g_{bf}$) interaction strengths and relative trap frequency [$\theta = (\omega_f/\omega_b)^2$]. Please note that, for the unperturbed mixture we have $g_b = 0.0$, $g_{bf} = 1.0$ and $\theta = 1.0$.

The computed $\gamma_{1i}^\sigma(x)$ for $g_b = 0.0$ and $g_{bf} = 0.8, 0.9, 1.0$ are presented in Supp-Fig. 9, where, as an exemplary result, the profiles of $\gamma_{11}^\sigma, \gamma_{13}^\sigma, \gamma_{15}^\sigma$ are depicted for the fermionic (upper panels) and bosonic (lower panels) species, respectively. These figures show the robustness of $\gamma_{1i}^\sigma(x)$. For the other two types of perturbations, similar observations hold according to Supp-Fig. 10, where the Bose-Bose interaction is solely varied with $g_b = 0.0, 0.1, 0.2$ and Supp-Fig. 11 where the relative trap frequencies are varied as $\theta = 0.9, 1.0, 1.1$.

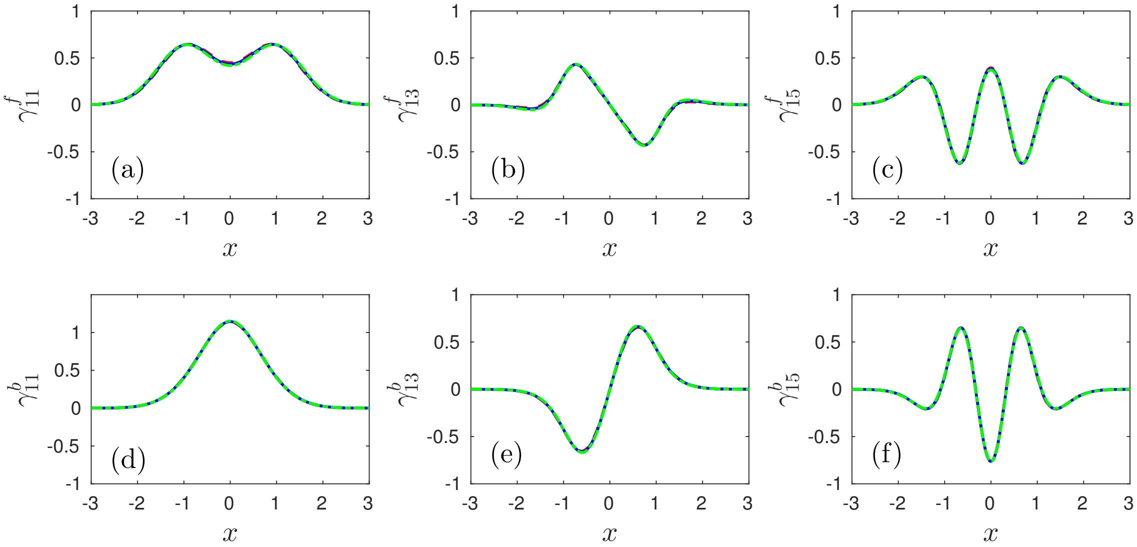


Supp-Fig. 9. $\gamma^{\sigma}_{1i}(x)$ for $g_{bf} = 0.8$ (red dashed line), $g_{bf} = 0.9$ (blue solid line) and $g_{bf} = 1.0$ (green dash-dot line) with $g_b = 0.0$ and $\theta = 1.0$. Upper (lower) panels are for fermionic (bosonic) species.

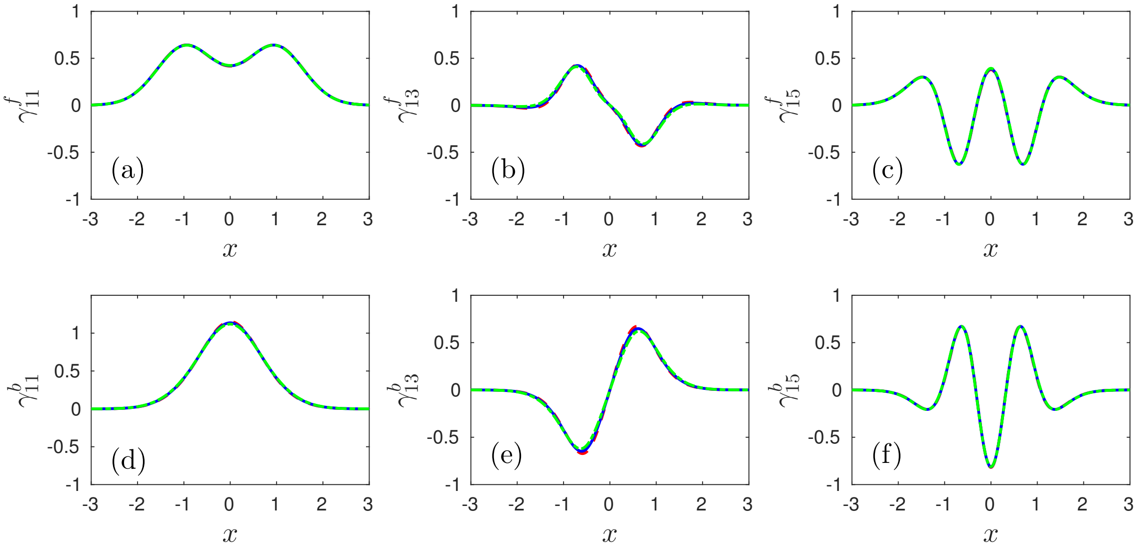


Supp-Fig. 10. $\gamma^{\sigma}_{1i}(x)$ for $g_b = 0.0$ (red dashed line), $g_b = 0.1$ (blue solid line) and $g_b = 0.2$ (green dash-dot line) with $g_{bf} = 1.0$ and $\theta = 1.0$. Upper (lower) panels are for fermionic (bosonic) species.

[1] L. Cao, V. Bolsinger, S. I. Mistakidis, G. M. Koutentakis, S. Krönke, J. M. Schurer and P. Schmelcher, J. Chem. Phys. **147**, 044106 (2017).
[2] L. Cao, S. Krönke, O. Vendrell, and P. Schmelcher, J. Chem. Phys. **139**, 134103 (2013).
[3] S. Krönke, L. Cao, O. Vendrell, and P. Schmelcher, New J. Phys. **15**, 063018 (2013).
[4] H.-D. Meyer, U. Manthe, and L. Cederbaum, Chem. Phys. Lett. **165**, 73 (1990).

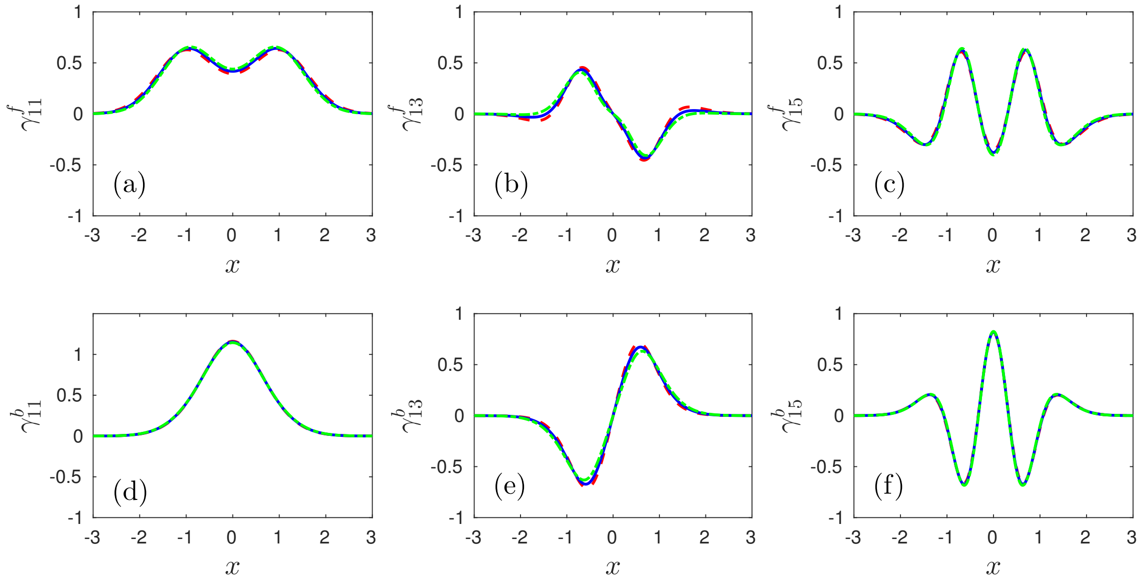


Supp-Fig. 11. $\gamma^{\sigma}_{1i}(x)$ for $\theta = 0.9$ (red dashed line), $\theta = 1.0$ (blue solid line) and $\theta = 1.1$ (green dash-dot line) with $g_{bf} = 1.0$ and $g_b = 0.0$. Upper (lower) panels are for fermionic (bosonic) species.
